# Supplementary material for: Inequivalence of Single-Particle and Population Lifetimes in a Cuprate Superconductor
Source: arXiv:1505.07512 source file (2015-05-27)
Supplement: Supplementary file 1 [file YangSL_Bi2212_scatteringRate_SM_3rdrev.pdf]

# Inequivalence of Single-Particle and Population Lifetimes in a Cuprate Superconductor - Supplemental Material

S.-L. Yang,[1,2] J. A. Sobota,[1,3] D. Leuenberger,[1,2] Y. He,[1,2] M. Hashimoto,[4]
D. H. Lu,[4] H. Eisaki,[5] P. S. Kirchmann,[1,*] and Z.-X. Shen[1,2,†]

[1]*Stanford Institute for Materials and Energy Sciences, SLAC National Accelerator Laboratory, 2575 Sand Hill Road, Menlo Park, CA 94025, USA*
[2]*Geballe Laboratory for Advanced Materials, Departments of Physics and Applied Physics, Stanford University, Stanford, CA 94305, USA*
[3]*Advanced Light Source, Lawrence Berkeley National Laboratory, Berkeley, CA 94720, USA*
[4]*Stanford Synchrotron Radiation Lightsource, SLAC National Accelerator Laboratory, 2575 Sand Hill Road, Menlo Park, California 94025, USA*
[5]*Electronics and Photonics Research Institute, National Institute of Advanced Industrial Science and Technology, Tsukuba, Ibaraki 305-8558, Japan*

(Dated: May 22, 2015)

## LIMITED DYNAMIC RANGE OF THE PHOTO-EXCITED HOLE POPULATION

Noise in photoemission experiments generally obeys Poisson statistics [1] and scales with the square root of the signal. In our experiment, the strong equilibrium spectrum below $E_\mathrm{F}$ introduces a considerable noise, which limits the detectable dynamic range of the photoexcited hole population. It is for this reason that we focus on the electron dynamics above $E_\mathrm{F}$ in the main text.

In Fig. S1 we demonstrate this technical limitation by plotting the background-subtracted signal above and below $E_\mathrm{F}$ near time zero. While the electron population is clearly above its noise level up to 80 meV, the hole population is overwhelmed by noise for $|E - E_\mathrm{F}| > 40$ meV. The limited dynamic range of the hole population does not allow a discussion on the lifetime near the characteristic energy $\sim 70$ meV.

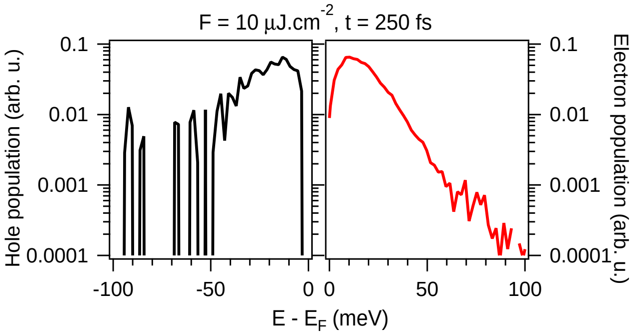


FIG. S1. Comparison of dynamic ranges for the electron (red) and hole (black) populations at 250 fs using an incident fluence of 10 $\mu$J.cm$^{-2}$ at 20 K. The dynamic range of the hole population is considerably smaller than that of the electron population due to the strong background-induced noise.

## INTENSITY CUTOFFS FOR THE POPULATION FITTING

As discussed in the main text, we define the fitting window using a 20% intensity cutoff ($\Delta I(t) > 20\%\Delta I_\mathrm{max}$). Fig. S2 shows that switching to a 10% or 30% cutoff has negligible impact on the fitted rates for all fluences and energies.

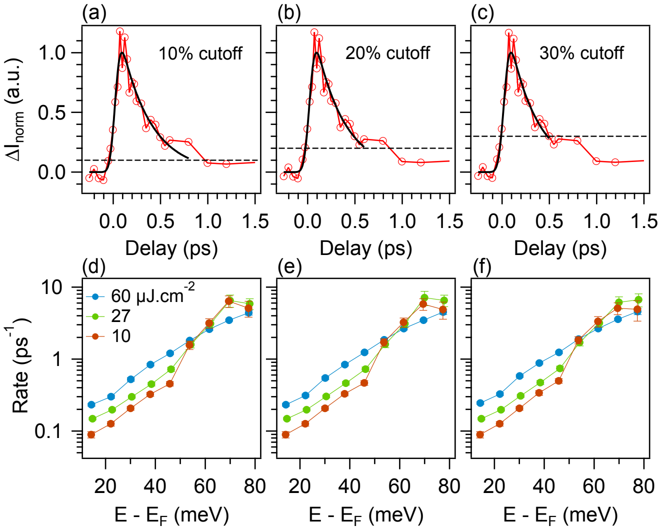


FIG. S2. Comparison of the fitted decay rates using different intensity cutoff values. (a)$\sim$(c) Exemplary fits ($F$ = 10 $\mu$J.cm$^{-2}$, $E$ - $E_\mathrm{F}$ = 62 meV, $T$ = 20 K) when defining the fitting window using intensity cutoffs at 10% (a), 20% (b), and 30% (c) of the peak value. (d)$\sim$(f) The corresponding fitting results for all fluences.

## ARPES SELF ENERGY ANALYSIS

In Fig. S3 we demonstrate how to obtain the imaginary part of self energy Im$\Sigma$ from the nodal ARPES cut

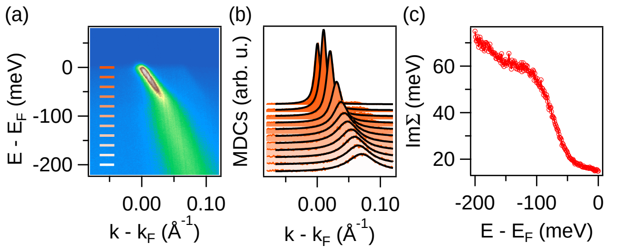


FIG. S3. ARPES self energy analysis. (a) nodal cut at 20 K. (b) Exemplary MDCs (orange shading) and Lorentzian fits (black lines) extracted from panel (a). (c) Extracted ImΣ by multiplying the MDC width with the bare-band velocity.

at 20 K. Momentum distribution curves (MDCs) are obtained for each energy (Fig. S3(a)). These MDCs are then fitted using Lorentzian functions (Fig. S3(b)). ImΣ is obtained by multiplying the half-width-half-maxima of the Lorentzian fits ($\Delta k$) with a bare-band velocity ($v_0$). $v_0$ is conventionally chosen to be the slope of the linear line connecting the dispersion at $E - E_\mathrm{F} = 0$ and $-200$ meV [2].

## ENERGY-INTEGRATED POPULATION DECAY RATE

To connect to the energy-integrated population dynamics measured by time-resolved reflectivity, we integrate the electron population from $E_\mathrm{F}$ to 200 meV and extract the decay rates as shown in Fig. S4. We find good agreement between our results and Ref. [3]: at temperatures far below $T_\mathrm{c}$ the decay rates are strongly fluence-dependent and drop below 0.1 ps$^{-1}$ at low fluences; at temperatures above $T_\mathrm{c}$ the decay rates are weakly fluence-dependent and settle at a value of $\sim$ 1.5 ps$^{-1}$. This agreement between time-resolved photoemission and reflectivity measurements was also observed in a previous study on Bi-2212 [4].

A notable feature in the energy-integrated rate at 20 K is a kink near 15 $\mu$J.cm$^{-2}$. This is the threshold fluence beyond which the superconducting gap is transiently melted, in agreement with previous measurements [5, 6].

## COLLISION INTEGRALS FOR ELECTRON-PHONON INTERACTIONS

In the main text we outline a general formalism to distinguish population lifetimes ($\tau_\mathrm{p}$) and single-particle lifetimes ($\tau_\mathrm{s}$). To apply this formalism to electron-phonon interactions, we specify the scattering probability $W_{\mathbf{k},\mathbf{k}'}$ as $\frac{2\pi}{\hbar} g^2_{\mathbf{k},\mathbf{k}'}[1 + n(\Omega)]$ for emitting a phonon of energy $\Omega$, and as $\frac{2\pi}{\hbar} g^2_{\mathbf{k},\mathbf{k}'} n(\Omega)$ for absorbing this phonon. Here $g_{\mathbf{k},\mathbf{k}'}$

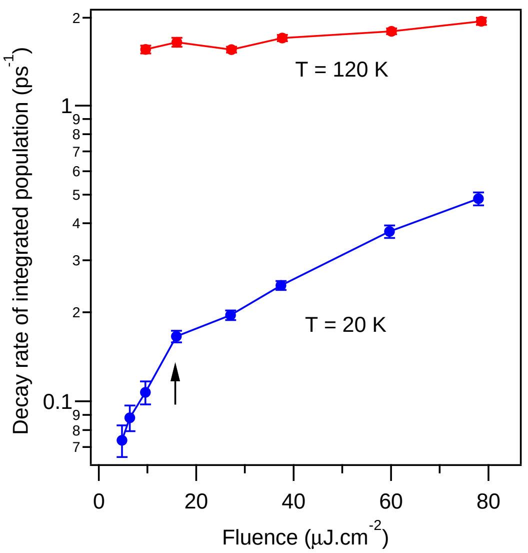


FIG. S4. Energy-integrated population decay rates for 20 K and 120 K. The arrow marks the threshold fluence beyond which the superconducting gap is transiently melted.

and $n$ stand for the coupling vertex and Bose-Einstein distribution, respectively.

$\tau_\mathrm{s}$ at the electronic state $\epsilon_\mathbf{k}$ is then expressed as:

$$\frac{1}{\tau_\mathrm{s}(\epsilon_\mathbf{k})} = \frac{2\pi}{\hbar}\int \frac{d\mathbf{k}'}{(2\pi)^3} g^2_{\mathbf{k},\mathbf{k}'}[1 - f(\epsilon_{\mathbf{k}'}) + n(\Omega)]\delta(\epsilon_\mathbf{k} - \epsilon_{\mathbf{k}'} - \Omega) + \frac{2\pi}{\hbar}\int \frac{d\mathbf{k}'}{(2\pi)^3} g^2_{\mathbf{k},\mathbf{k}'}[f(\epsilon_{\mathbf{k}'}) + n(\Omega)]\delta(\epsilon_\mathbf{k} - \epsilon_{\mathbf{k}'} + \Omega) \quad \text{(S1)}$$

Eqn. S1 is precisely the single-particle lifetime as derived in many textbooks [7, 8]. The difference between $1/\tau_\mathrm{p}$ and $1/\tau_\mathrm{s}$ can be similarly derived as:

$$\frac{1}{\tau_\mathrm{p}(\epsilon_\mathbf{k})} = \frac{1}{\tau_\mathrm{s}(\epsilon_\mathbf{k})} - \frac{2\pi}{\hbar}\int \frac{d\mathbf{k}'}{(2\pi)^3} g^2_{\mathbf{k},\mathbf{k}'}[f(\epsilon_\mathbf{k}) + n(\Omega)] \times\delta(\epsilon_\mathbf{k} - \epsilon_{\mathbf{k}'} - \Omega)\frac{\delta f(\epsilon_\mathbf{k} - \Omega)}{\delta f(\epsilon_\mathbf{k})} - \frac{2\pi}{\hbar}\int \frac{d\mathbf{k}'}{(2\pi)^3} g^2_{\mathbf{k},\mathbf{k}'}[1 - f(\epsilon_\mathbf{k}) + n(\Omega)] \times\delta(\epsilon_\mathbf{k} - \epsilon_{\mathbf{k}'} + \Omega)\frac{\delta f(\epsilon_\mathbf{k} + \Omega)}{\delta f(\epsilon_\mathbf{k})} \quad \text{(S2)}$$

Without loss of generality we focus on the electron dynamics ($\epsilon_\mathbf{k} > 0$). In the low-temperature limit, $f(\epsilon_\mathbf{k})$ and $n(\Omega)$ at finite $\epsilon_\mathbf{k}$ and $\Omega$ both vanish. In Eqn. S2, the first integral which describes the interaction with excitations at $\epsilon_\mathbf{k} - \Omega$ is thus negligible. In the low-fluence limit, the photoexcited population vanishes exponentially as a

function of energy (Fig. S1). The second integral which describes the interaction with excitations at $\epsilon_{\mathbf{k}}+\Omega$ is also negligible due to the vanishing $\delta f(\epsilon_{\mathbf{k}}+\Omega)/\delta f(\epsilon_{\mathbf{k}})$.

Therefore, for electron-phonon scattering $\tau_{\mathrm{p}}$ converges to $\tau_{\mathrm{s}}$ in the low-temperature, low-fluence limit.

---

* kirchman@slac.stanford.edu
† zxshen@stanford.edu

[1] D. L. Fried, Applied Optics **4**, 79 (1965).
[2] W. S. Lee *et al.*, Phys. Rev. B **77**, 140504 (R) (2008).
[3] N. Gedik *et al.*, Phys. Rev. B **70**, 014504 (2004).
[4] C. L. Smallwood *et al.*, Science (New York, N.Y.) **336**, 1137 (2012).
[5] C. L. Smallwood *et al.*, Phys. Rev. B **89**, 115126 (2014).
[6] W. Zhang *et al.*, Phys. Rev. B **88**, 245132 (2013).
[7] G. Grimvall, *The Electron-Phonon Interaction in Metals* (North-Holland Pub. Co., Amsterdam, 1981).
[8] G. D. Mahan, *Many-Particle Physics (Physics of Solids and Liquids)* (Springer, 2000).
